# Supplementary material for: Non-monotone Submodular Maximization with Nearly Optimal Adaptivity and Query Complexity
Source: arXiv:1808.06932 source file (2023-04-07)
Supplement: Supplementary file 1 [file appendix-threshold.tex]

%\section{Missing Analysis from \Cref{sec:threshold}}
%\label{app:reduced-mean}

\section{Analysis of the \AdaptiveSampling Algorithm}
\label{app:analysis_adaptive_sampling}
In our analysis of the approximation factor of \NonmonotoneMaximization,
we use an inequality derived from part of the analysis of
\Cref{lem:adaptive_sampling}.
We note that all lemmas in this section are restatements borrowed
from~\cite{fahrbach2018submodular}, and we include them here for the sake of
completeness.
%We start by restating the some preliminary lemmas. 

%To prove the guarantees of \AdaptiveSampling (\Cref{lem:adaptive_sampling}), we
%first give a result that demonstrates the monotonic behavior of $\cD_t$ at any
%point in the algorithm.  This is a simple consequence of submodularity and the
%proof can be found in \Cref{app:nonincreasing_proof}.

\begin{lemma}[\cite{fahrbach2018submodular}]
\label{lem:percentage_nonincreasing}
In each round of \AdaptiveSampling,
$\E[I_1] \ge \E[I_2] \ge \dots \ge \E[I_{|A|}]$.
\end{lemma}

\begin{lemma}[\cite{fahrbach2018submodular}]
\label{lem:filter}
In each round of \AdaptiveSampling, an expected $\hat{\varepsilon}$-fraction
of $A$ is filtered with probability at least $1 - \hat{\delta}$.
\end{lemma}

\begin{lemma}[\cite{fahrbach2018submodular}]
\label{lem:filters-all}
If \AdaptiveSampling terminates with $|S| < k$, then
$|A| = 0$ with probability at least $1 - \delta$.
\end{lemma}

Using the guarantees for \EstimateMean and
the two lemmas above, we can prove \Cref{lem:adaptive_sampling}.

\begin{proof}[
  Proof of \Cref{lem:adaptive_sampling}~\textnormal{(\cite{fahrbach2018submodular})}]
We start by showing the adaptivity complexity of \AdaptiveSampling is
$O(\log(n/\delta)/\varepsilon)$.
By construction,
the number of rounds is $O(\log_{(1-\varepsilon)^{-1}}(n/\delta))$
and there are polynomially-many queries in each, all of which are independent
and rely on the current state of~$S$.

To prove the three properties, we use \Cref{lem:filters-all} to assume
that with probability at least $1 - \delta$ all $O(rm)$ calls to \EstimateMean yield
correct outputs, and also that if the algorithm terminates with $|S| < k$ then
we have $|A| = 0$.
For the Property 1, the total number of oracle queries incurred by calling
\EstimateMean is
  $O\parens{rm\log\parens*{\delta^{-1}}/\varepsilon^{2}}
  = 
  O\parens{\log\parens*{n/\delta}\log\parens*{k}\log\parens*{\delta^{-1}}/\varepsilon^4}$
by \Cref{lem:estimator}.
Note that we can sample from $\mathcal{D}_t$ with two oracle calls.
Now we bound the expected number of queries made while filtering over
the course of the algorithm. Let $A_i$ be a random variable for the value
of $A$ in the $i$-th round. It follows from the geometric property
$\E[|A_{i+1}|] \le (1 - \hat\varepsilon) \cdot \E[|A_i|]$ in
the proof of \Cref{lem:filters-all} and by linearity that the expected number of
queries is bounded by
\begin{align*}
  \Exp{}{\sum_{i=0}^r \abs*{A_{i}}} = \sum_{i=0}^r \Exp{}{\abs*{A_i}}
  \le n \sum_{i=0}^r \parens*{1 - \hat\varepsilon}^i
  \le n/\hat\varepsilon.
\end{align*}
Since we set $\delta^{-1} = O(\poly(n))$, the number of expected
queries made when filtering dominates the sum of queries made when calling
\EstimateMean.

For property 2,
it suffices to lower bound the expected marginal of
every element added to $S$ if we
think of adding each set $T$ to the output $S$
one element at a time according to a uniformly random permutation.
Let $t^* = \min\{t, k-|S|\}$ be the size of $T$ at an arbitrary
round.
If $t^* = 1$ then $\E[\Delta(T,S)] \ge \tau$ by the definition of $A$.
Otherwise, the candidate size $t \ge t^*/(1+\hat\varepsilon)$
in the previous iteration
has the property that $\E[I_t] \ge 1 - 2\hat\varepsilon$.
Since $T \sim \mathcal{U}(A,t^*)$ uniformly at random, we can lower bound the
expected marginal $\E[\Delta(T,S)]$ by the contribution of the
first $t$ elements, giving us
\begin{align}\label{eq:AvgValLB}
  \Exp{}{\Delta(T,S)} &\ge
  \parens*{\Exp{}{I_1} + \Exp{}{I_2} + \dots + \Exp{}{I_{t}}}\tau \nonumber\\
  &\ge t (1-2\hat\varepsilon) \tau \\
  &\ge \frac{t^*}{1+\hat\varepsilon} \cdot (1-2\hat\varepsilon)\tau \nonumber\\
  &\ge t^*(1-\varepsilon) \tau.\nonumber
\end{align}
The first of the inequalities above uses the definition of $I_t$ in
\Cref{def:indicator_distribution} and is analogous to Markov's inequality,
and the second follows from \Cref{lem:percentage_nonincreasing}.
Since the expected marginal of any individual element is at least
$(1-\varepsilon)\tau$, we have Property 2.

To show Property 3, recall that if the algorithm terminates with $|S| < k$,
then we have $|A| = 0$ with probability at least $1 - \delta$ by
\Cref{lem:filters-all}.
Therefore, it follows from the definition of $A$ and submodularity
that $\Delta(x,S) < \tau$ for all $x \in N$.
\end{proof}
